# Supplementary material for: Network Binarization via Contrastive Learning
Source: arXiv:2207.02970 source file (2022-07-16)
Supplement: Supplementary file 1 [file 8Appendix.tex]

\section{Appendix}
\subsection{CMIM Algorithm}
\begin{algorithm}[!h] 
\caption{Forward and Backward Propagation of CMIM}  
\label{alg:MIM}
% \vspace*{-4mm}
\begin{multicols}{2}
\begin{algorithmic}[1] 
	\Require A minibatch of data samples $(\mathbf{X,Y})$, current binary weight $\mathbf{W}_B^k$, latent full-precision weights $\mathbf{W}_F^k$, and learning rate $\eta$.
	\Ensure Update weights ${\mathbf{W}_F^k}^{\prime}$.
	\State \textbf{Forward Propagation}:
    \For{$k = 1$ to $K-1$}
    \State Binarize latent weights: $\mathbf{W}_B^k \xleftarrow{} \mathrm{sgn}(\mathbf{W}_F^k)$;
    	\State Perform binary operation with the activations of next layer:
    	$\mathbf{A}_F^{k} \xleftarrow{} \mathrm{XnorDotProduct}(\mathbf{W}_B^k, \mathbf{A}_B^{k-1})$;
    	\State Perform Batch Normalization: $\mathbf{A}_F^{k} \xleftarrow{} \mathrm{BatchNorm}(\mathbf{A}_F^{k})$;
    	\State Binarize full-precision activations and obtain binary ones : $\mathbf{A}_B^k \xleftarrow{} \text{sgn}(\mathbf{A}_F^k)$;
    \EndFor
    \State For $k = 1,\cdots, K$, pair $\left\{\mathbf{a}_B^{k,i}\right\}$ and $\left\{\mathbf{a}_B^{k,j}\right\}$ as negative and positive pairs, then use Eq.~\ref{eq:loss1} layer by layer to compute the NCE loss $\mathcal{L}^{k}_{NCE}$ between $\mathbf{A}_B^{k}$ and $\mathbf{A}_F^{k}$ for contrastive learning;
    \State Combine a series of NCE loss $\left\{\mathcal{L}^{k}_{NCE}\right\}$ with the classification loss $\mathcal{L}$ into the CMIM loss $\mathcal{L}_{CMIM}$, with Eq.~\ref{eq:loss2};
	\State \textbf{Backward Propagation}:
    compute the gradient of the overall loss function, \textit{i.e.}~$\frac{\partial\mathcal{L}}{\partial \mathbf{W_B}}$, using the STE to handle the sign function;
	\State \textbf{Parameter Update}:~update the full-precision weights: ${\mathbf{W}_F^i}^{\prime} \xleftarrow{} \mathbf{W}_F^k - \eta \frac{\partial\mathcal{L}}{\partial \mathbf{W}_B^k}$.
\end{algorithmic}  
\end{multicols}
\vspace*{-2mm}
\end{algorithm}

\subsection{Experimental Results of CAD \& WCoRD on BNNs}
Utilizing additional full-precision networks as teachers, we experimentally implement those contrastive-based knowledge distillation methods (\textit{i.e.} CRD~\cite{tian2019contrastive} and WCoRD~\cite{chen2021wasserstein}) into the binarization task, and we observe that CRD scales poorly on BNNs. 
In particular, we use CRD and WCoRD in a standard way (\textit{i.e.} $\mathcal{L} = \lambda\cdot\mathcal{L}_{CRD}  + \mathcal{L}_{cls}$ and $\mathcal{L} = \lambda\cdot\mathcal{L}_{WCoRD}  + \mathcal{L}_{cls}$), and we fine-tune the models by adjusting the hyper-parameter $\lambda$ in the loss function.
Table~\ref{table:crd} shows that a naive extension preforms much worse than our proposed version (we only report the best results \textit{w.r.t.} $\lambda$). 
In fact, straight-forwardly introducing a FP network as a teacher has already been comprehensively studied in Training Binary Neural Networks with \textbf{Real-to-Binary} Convolutions (ICLR 2020). In this work, Martinez \textit{et al.} points out that the existing KD methods can not be easily generalized into BNN mainly because of the huge differences between full-precision and binary weights and activations. In practice, this inconsistency hinders the binary and full-precision representations to be aligned within the knowledge distillation framework. Note that more detailed comparisons between ours and CRD are discussed in Section 3.3 (L408-432).
% regardless the extra requirement for full-precision network as teacher.
\begin{table}[!t]
\centering
    % \captionsetup{font=small}
    \caption{Top-1 accuracy (\%) on CIFAR-10 (C-10) and CIFAR-100 (C-100) test set. The higher the better. W/A denotes the bit number of weights/activations. }
    \scalebox{0.7}{
    \begin{tabular}{ccccc}
        \toprule
        \multirow{2}{*}{Topology}  & \multirow{2}{*}{Method}    & Bit-width       & Acc.(\%)  & Acc.(\%)     \\
                             &                & (W/A)           & (C-10)  & (C-100)      \\ \hline
                             & IR-Net ~\cite{qin2020forward}  & 1/1             & 91.6   & 64.5       \\
                             & RBNN ~\cite{lin2020rotated}  & 1/1             & 92.2   & 65.3      \\\cline{2-5}
                             & IR-Net + CRD~\cite{tian2019contrastive}  & 1/1             & 91.2   & 64.2       \\
     ResNet                  & RBNN + CRD~\cite{tian2019contrastive}  & 1/1             & 91.7   & 65.0      \\\cline{2-5}
      -18                    & IR-Net + WCoRD~\cite{chen2021wasserstein}     & 1/1             & 91.3   & 64.1       \\
                             & RBNN + WCoRD~\cite{chen2021wasserstein}  & 1/1             & 91.5   & 65.0      \\\cline{2-5}
                             & IR-Net + CMIM   & 1/1             & \textbf{92.2}  & \textbf{71.2}     \\ 
                             & RBNN + CMIM      & 1/1             & \textbf{92.8}  & \textbf{71.4}     \\ \bottomrule
    \end{tabular}}
    \label{table:crd}
\end{table}
